# Supplementary material for: Spectral Signatures of Non-Trivial Topology in a Superconducting Circuit
Source: arXiv:2401.10876 source file (2024-11-25)
Supplement: Supplementary file 1 [file suppfig_susy.pdf]

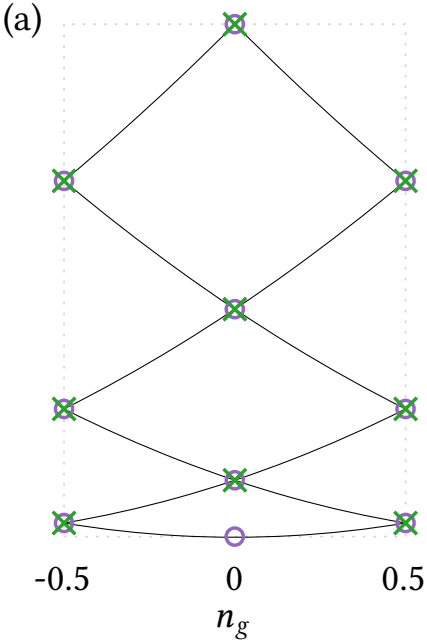

(b)  $n_g = 0, \text{Tr } P = 1$

$$|m_{\pm}\rangle = \frac{1}{\sqrt{2}}(|m\rangle \pm | -m \rangle)$$

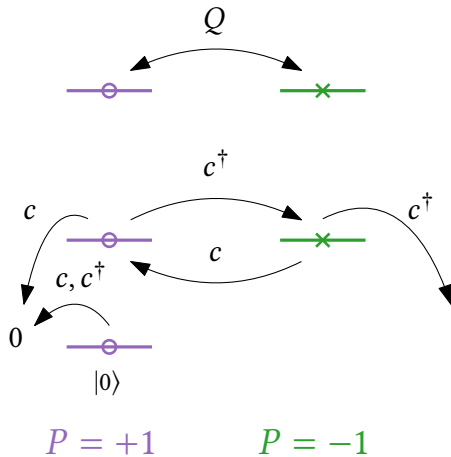

(c)  $n_g = +1/2, \text{Tr } P = 0$

$$|m_{\pm}\rangle = \frac{1}{\sqrt{2}}(|m\rangle \pm | -m + 1 \rangle)$$

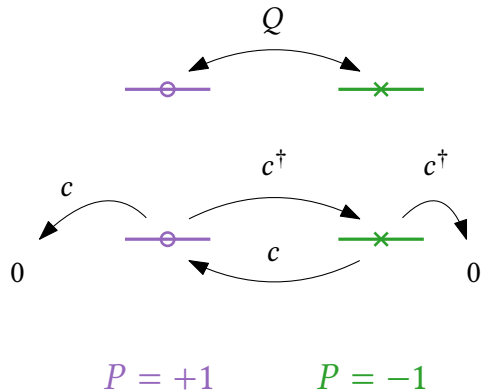

$$Q = \sqrt{E_C}(\hat{n} - n_g)$$

$$P = \sum_n | -n + 2n_g \rangle \langle n |$$

$$c = \frac{1 + P}{2} Q$$

$$-\frac{1}{2}$$

$$\begin{matrix} 0 \\ n_g \end{matrix}$$

$$\frac{1}{2}$$

(a)

(b)

(c)
